# Supplementary material for: Pix3D: Dataset and Methods for Single-Image 3D Shape Modeling
Source: arXiv:1804.04610 source file (2018-04-12)
Supplement: Supplementary file 1 [file pair_sample.tex]

\begin{figure}[t]
\centering
\includegraphics[trim={0 1.5cm 0 5cm},clip,width=\linewidth]{fig/pair_sample.pdf}
\caption{Sample Image and Shape Pair}
\label{fig:pair_sample}
\end{figure}
